# Supplementary material for: Towards photoassociation processes of ultracold rubidium trimers
Source: arXiv:2102.04779 ancillary file (2021-02-09)
Supplement: Supplementary file 1 [file Supplementary.pdf]

# Supplementary Material: Towards photoassociation processes of ultracold rubidium trimers

## COMPUTATIONAL DETAILS

### Basis set

In quantum chemistry molecular orbitals (MOs) are typically approximated by the *linear combination of atomic orbitals (LCAO)* ansatz, i.e.

$$\phi_i(\mathbf{r}) = \sum_{\mu} c_{i,\mu}\chi_\mu(\mathbf{r})\,. \tag{S1}$$

Here it is assumed that MOs ($\phi_i$) are similar to atomic orbitals (AOs) ($\chi_\mu$) close to the nuclei and interpolate between two AOs in-between two nuclei. Given this basis set expansion with basis functions $\chi_\mu$ the question arises how to choose them meaningfully. In practice Gaussian-type orbitals (GTOs)

$$\chi_\mu^{\mathrm{GTO}}(\mathbf{r}) \propto \exp(-\zeta|\mathbf{r}-\mathbf{R}_0|^2)\,, \tag{S2}$$

with $\mathbf{R}_0$ the center of the Gaussian usually placed at the coordinates of a nucleus, are commonly used as they allow for efficiently computing (analytically – keyword *Gaussian product theorem*) emerging integrals (each additionally multiplied by $Y_{l,m}r^{n-1}$, with the spherical harmonics $Y_{l,m}$) with existing fast and stable algorithms. However, this comes at the cost of physical meaningfulness since GTOs fail in describing the cusp at the nuclei and decay too quickly at long range. It turns out, however, that the correct physical behaviour can be fitted to a very good approximation by a linear combination of a sufficiently large number of GTOs with different, so called, exponents $\zeta$. That is, every function corresponding to a given $l$ quantum number comes with a certain number of exponents, i.e.

$$\chi_\mu^{nlm}(\mathbf{r},\theta,\phi;\mathbf{R}_0) = \frac{1}{N}Y_{lm}(\theta,\phi)(\mathbf{r}-\mathbf{R}_0)^{n-1}\sum_{i=1}^{P} w_i \exp\left(-\zeta_i(\mathbf{r}-\mathbf{R}_0)^2\right)\,. \tag{S3}$$

Here, $w_i$ describing the contraction coefficients which are usually introduced to avoid that the number of basis functions grows too large. With that the GTOs are combined in pre-defined linear combinations. Note that in quantum chemical calculations the exponents $\zeta_i$ and contractions coefficients $w_i$ are kept fix; only the MO coefficients $c_{i,\mu}$ are varied. The basis set parameters $\zeta_i$ and $w_i$ are pre-determined in atomic calculations. Nevertheless, the basis set is still finite which is why we are faced with basis set superposition errors (BSSEs). To keep them as low as possible we construct a large uncontracted (i.e. without pre-defined linear combinations) basis set from a given valence basis set designed for a small-core ECP [S1]. This basis set was originally optimized with respect to the polarizability thus providing not enough diffuse functions (i.e. small values of $\zeta$ thus high spread of corresponding function) for a proper description of loosely bound electrons as, e.g., in higher electronic states [S2]. Analogously to the basis set construction approach by Soldán in Ref. [S3] for the quartet ground state of $Rb_3$, we first add a $(2s, 2p, 2d, 2f)$ set of diffuse functions to the previously mentioned basis set (i.e. two additional diffuse $s$-exponents, etc.). Secondly we calculate within this resulting span of functions new exponents in an even-tempered manner (i.e. resulting exponents form a geometric series, in other words they are evenly spaced in logarithmic representation) and finally generate additional $g$-exponents (i.e. additional polarization functions) using

$$\zeta^\ell = \zeta^0\frac{\ell+3}{3} \tag{S4}$$

as it was proposed in Ref. [S4–S6] resulting in a $[15s12p7d5f3g]$ uncontracted even-tempered basis set ($\equiv$ UET15). The $g$-exponents are added to account as well as possible for deviations of the orbitals from the sperical shape (so do the $d$- and $f$-exponents). In Ref. [S7] it has been shown that even-tempered basis sets span the Hilbert space evenly and provide a way for accurately simulate fully optimized exponents without optimizing any of them. The corresponding exponents are listed in Tab. S.I.

Table S.I. Exponents $\zeta_i$ of the 15s12p7d5f3g uncontracted even-tempered basis set (UET15) constructed for this work (see main text). Here we have 15 exponents for describing $s$ orbitals, 12 for the description of $p$ orbitals and so on.

| Exponents | | | | |
|---|---|---|---|---|
| s | p | d | f | g |
| 240.216 800 | 46.597 790 | 1.750 670 | 2.431 530 | 2.836 785 |
| 105.929 280 | 17.646 390 | 0.614 850 | 0.714 329 | 0.833 384 |
| 46.712 021 | 6.682 615 | 0.215 940 | 0.209 854 | 0.244 830 |
| 20.598 771 | 2.530 679 | 0.075 840 | 0.061 650 | |
| 9.083 515 | 0.958 358 | 0.026 636 | 0.018 112 | |
| 4.005 591 | 0.362 926 | 0.009 355 | | |
| 1.766 360 | 0.137 439 | 0.003 285 | | |
| 0.778 918 | 0.052 047 | | | |
| 0.343 482 | 0.019 710 | | | |
| 0.151 467 | 0.007 464 | | | |
| 0.066 793 | 0.002 827 | | | |
| 0.029 454 | 0.001 070 | | | |
| 0.012 988 | | | | |
| 0.005 728 | | | | |
| 0.002 526 | | | | |

## Active space

We have choosen an active space of 5/4/2/1 (according to the internal odering $(A_1/B_1/B_2/A_2)$ for the $C_{2v}$ point group in MOLPRO) which comprises the $5s$ and $5p$ $(p_x, p_y, p_z)$ orbitals of the three Rb atoms. Consequently, our active space describes three electrons in 12 orbitals.

## Accuracy of the method – Rb energy levels

Our computational approach involves MRCI with large-core effective core potential (ECP) in combination with a core polarization potential (CPP). At this the large-core ECP has been fitted to experimental values of atomic Rb energy levels [S8], as it is described in the main text. Thus, unsurprisingly, those values are reproduced very accurately as shown in Tab. S.II.

Table S.II. Comparison of calculated Rb energy levels and their relative splittings with experimental data from the NIST [S9] database. Calculations are performed at the MRCI(ECP+CPP)/15s12p7d5f3g level of theory.

| Term | $J$ | Absolute levels [cm$^{-1}$] | | Level splittings [cm$^{-1}$] | |
|---|---|---|---|---|---|
| | | this work | NIST | this work | NIST |
| $^2$S | 1/2 | | 0 | | |
| $^2$P | 1/2 | 12577.76 | 12578.95 | 12577.76 | 12578.95 |
| | 3/2 | 12811.80 | 12816.55 | 234.04 | 237.60 |
| $^2$D | 5/2 | 19356.95 | 19355.20 | 6545.15 | 6538.66 |
| | 3/2 | 19357.15 | 19355.65 | 0.20 | 0.45 |

## POSSIBLE CONFIGURATIONS OF THE TRIMER SYSTEM

For non-linear arrangements, the three atoms always define a plane and the electronic states can be characterized according to their symmetry with respect to the plane ($C_s$ point group symmetry, cf. Fig. S1 right bottom). The electronic wavefunction is either symmetric, irreducible representation (IRREP) $A'$, or antisymmetric (IRREP $A''$) with respect to this plane. Wavefunctions of different symmetry do not mix and their corresponding potential energy surfaces can intersect. There are special subspaces in the configurational space, in which the point group symmetry is higher. Still assuming non-linear geometries, if two interatomic distances are equal (isosceles triangle, cf. Fig. S1 left bottom), there are additional symmetry elements in the system (second mirror plane, point group $C_{2v}$) and if all three distances are equivalent, the point group is $D_{3h}$ (particular symmetry element: three-fold axis, cf. Fig. S1 left top). All these additional symmetries mean that states that belong to the same IRREP in $C_s$ can have different behavior with respect to the new symmetry elements and thus fall into different IRREPs. In this case, the associated potential energy surfaces can intersect in the high symmetry subspace, but mix (and thus avoid each other) in the adjacent low symmetry configurations.

For linear systems (cf. Fig. S1 right top), the symmetry is further increased (full cylindrical symmetry). A particular subtlety is the mixing of rotational and vibrational degrees of freedom, as at linear geometry only two (nuclear) rotational degrees of freedom exist, while a fourth vibrational degree of freedom comes into play. The "bending mode" of the molecule is twofold degenerate, while the molecular plane becomes undefined. Anomalies, like the Renner-Teller effect, are expected.

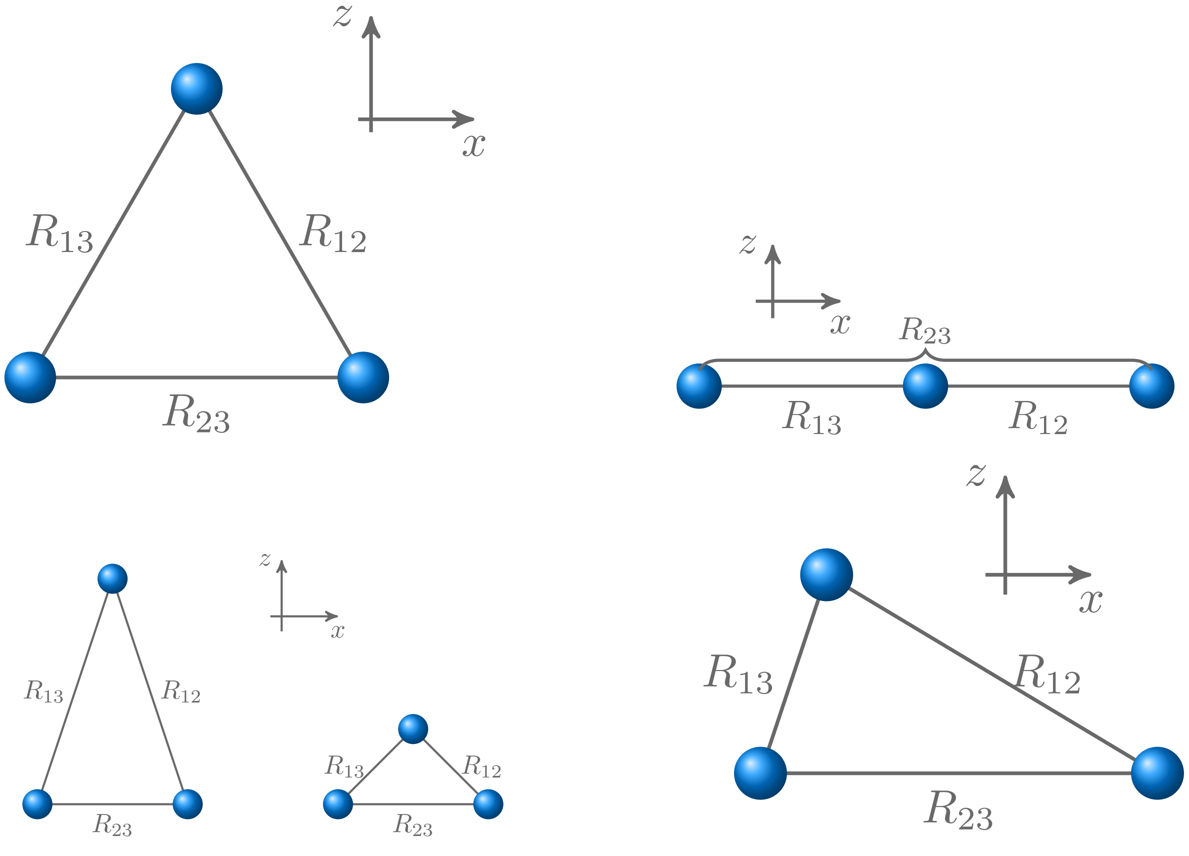


Figure S1. The $Rb_3$ system appears in three different special configurations (from left to right, top to bottom): Equilateral triangle described by the point group $D_{3h}$, equilateral linear configuration with full cylindrical symmetry represented by the $D_{\infty h}$ group and isosceles triangular configuration described by the $C_{2v}$ point group. In general, the three atoms always define a plane, i.e. if $R_{12} \neq R_{23} \neq R_{13}$ the system belongs to the point group $C_s$.

## OVERVIEW ON DOUBLET AND QUARTET STATES OF $RB_3$

In addition to what is shown in the main text where we only discuss classified global/ local minima of doublet and quartet states of $Rb_3$, we give a more detailed overview here. For this purpose we show all states up to the $5s + 2 \cdot 5p$ asymptote in Fig. S2. The corresponding numbers and classifications are listed in Tab. S.III for triangular configurations and in Tab. S.IV for linear geometries. Due to numerical difficulties in the frequency calculation at MRCI level of theory we were faced with convergence problems for some high-lying states and/or close-in-energy to other states wherefore we labelled them with »true classification failed«in Tabs. S.III and S.IV. This means that they could turn out as minimum or saddle points. We are only sure that they are extremal points on the corresponding PESs.

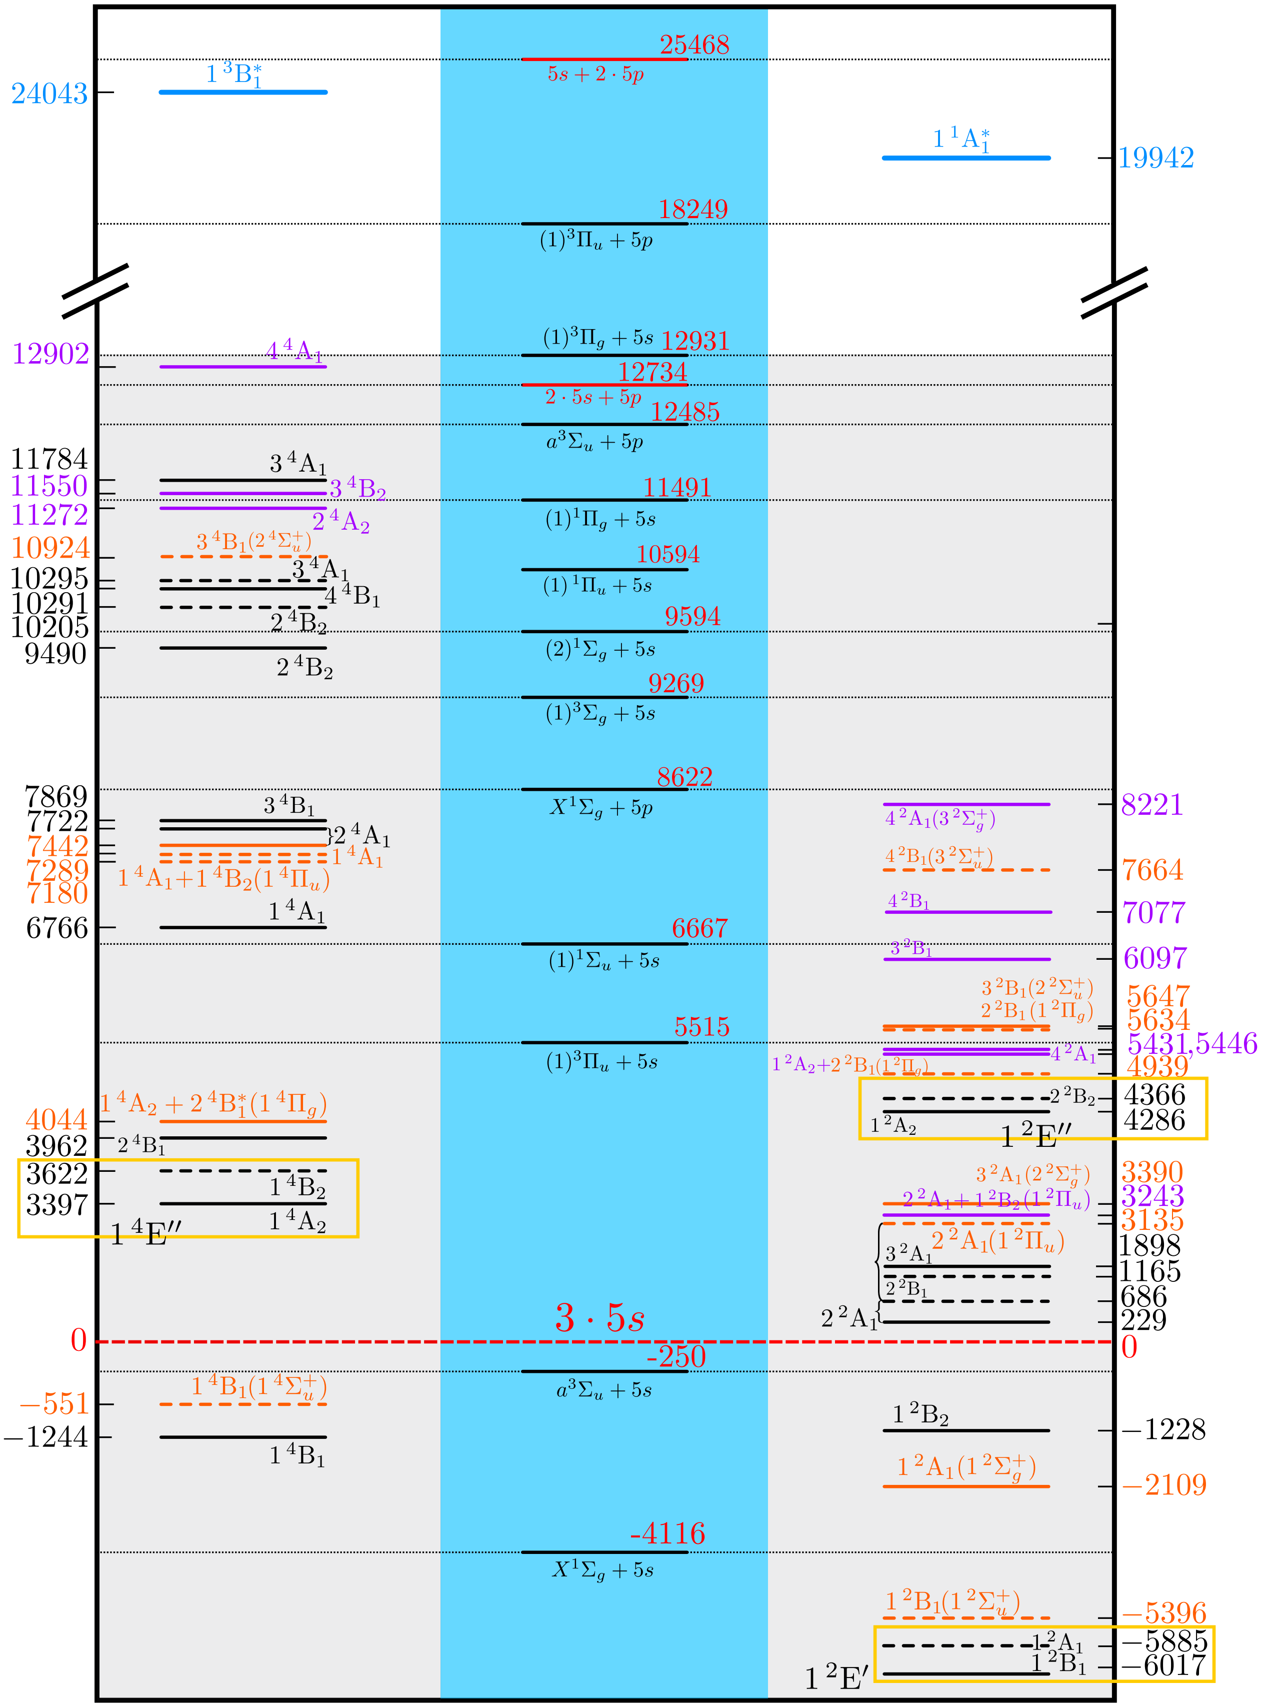


Figure S2. Overview of the energy levels of all doublet and quartet states of $Rb_3$ listed in Tab. S.III and S.IV. Black levels corresponding to triangular minima, orange levels are linear minima and levels given in purple corresponding to states (linear or triangular) for which the true three-dimensional classification failed. First-order saddle points are represented by dashed lines (both for linear and triangular geometries). In case of a degenerate Renner-Teller pair (e.g. $1\,^4A_2 + 2\,^4B_1^*$) the asterisks shows that this state turns out as first-order saddle point. Examples of Jahn-Teller pairs are highlighted by yellow boxes surrounding the corresponding states – a complete overview is given in Tab. S.V.

Table S.III. Synopsis of **triangular** ($C_{2v}$ and $D_{3h}$) doublet and quartet (ground and excited) states of $Rb_3$ as well as the singlet state of $Rb_3{}^+$ computed at MRCI(ECP+CPP)/UET15 level of theory.

| State ($D_{3h}$) | $R_{12}, R_{23}, R_{13}$ [Å] ($R_1, R_2, R_3$) | Geometry | $E_{\rm rel}$ [cm$^{-1}$] | Classification |
|---|---|---|---|---|
| $1\,^4B_1$ ($1\,^4A_2'$) | $5.311, 5.311, 5.311$ ($2.656, 2.656, 2.656$) | $D_{3h}$ | -1244 | Minimum |
| $1\,^4A_2$ ($1\,^4E''$) | $4.368, 5.700, 4.368$ ($1.518, 2.850, 2.850$) | $C_{2v}$ | 3397 | Minimum |
| $1\,^4B_2$ ($1\,^4E''$) | $4.913, 4.146, 4.913$ ($2.840, 2.073, 2.073$) | $C_{2v}$ | 3622 | First-order saddle point imag. freq. asymmetric stretch mode |
| $2\,^4B_1$ ($1\,^4E'$) | $4.442, 8.179, 4.442$ ($0.352, 4.090, 4.090$) | $C_{2v}$ | 3962 | Minimum |
| $1\,^4A_1$ upper ($1\,^4E'$) | $4.993, 8.076, 4.993$ ($0.955, 4.038, 4.038$) | $C_{2v}$ | 6766 | Minimum |
| $2\,^4A_1$ ($1\,^4A_1'$) | $5.325, 5.325, 5.325$ ($2.663, 2.663, 2.663$) | $D_{3h}$ | 7722 | Minimum |
| $3\,^4B_1$ ($2\,^4A_2'$) | $5.084, 5.084, 5.084$ ($2.542, 2.542, 2.542$) | $D_{3h}$ | 7869 | Minimum |
| $2\,^4B_2$ ($2\,^4E''$) | $4.443, 6.217, 4.443$ ($1.335, 3.109, 3.109$) | $C_{2v}$ | 9490 | Minimum |
| $2\,^4B_2$ upper ($2\,^4E''$) | $5.476, 4.207, 5.476$ ($3.373, 2.104, 2.104$) | $C_{2v}$ | 10205 | First-order saddle point imag. freq. symmetric stretch mode |
| $4\,^4B_1$ ($2\,^4E'$) | $5.283, 5.337, 5.283$ ($2.615, 2.669, 2.669$) | $C_{2v}$ | 10291 | Minimum |
| $3\,^4A_1$ lower ($2\,^4E'$) | $5.318, 5.279, 5.318$ ($2.679, 2.640, 2.640$) | $C_{2v}$ | 10295 | First-order saddle point imag. freq. asymmetric stretch mode |
| $2\,^4A_2$ ($2\,^4E''$) | $4.924, 4.874, 4.924$ ($2.487, 2.437, 2.437$) | $C_{2v}$ | 11272 | Local $C_{2v}$ extremum, true classification failed |
| $3\,^4B_2$ ($1\,^4A_2''$) | $4.619, 4.619, 4.619$ ($2.310, 2.310, 2.310$) | $D_{3h}$ | 11550 | Local $C_{2v}$ extremum, true classification failed |
| $3\,^4A_1$ upper ($2\,^4E'$) | $4.687, 7.226, 4.687$ ($1.074, 3.613, 3.613$) | $C_{2v}$ | 11784 | Minimum |
| $4\,^4A_1$ ($3\,^4E'$) | $4.862, 6.126, 4.862$ ($1.799, 3.063, 3.063$) | $C_{2v}$ | 12902 | Local $C_{2v}$ extremum, true classification failed |
| $1\,^2B_1$ ($1\,^2E'$) | $4.379, 5.393, 4.379$ ($1.682, 2.697, 2.697$) | $C_{2v}$ | -6017 | Minimum |
| $1\,^2A_1$ ($1\,^2E'$) | $4.863, 4.197, 4.863$ ($2.765, 2.096, 2.096$) | $C_{2v}$ | -5885 | First-order saddle point imag. freq. asymmetric stretch mode |
| $1\,^2B_2$ ($1\,^2A_2''$) | $4.276, 4.285, 4.276$ ($2.134, 2.143, 2.143$) | $C_{2v}$ | -1228 | Minimum |
| $2\,^2A_1$ lower ($2\,^2E'$) | $4.398, 6.073, 4.398$ ($1.361, 3.037, 3.037$) | $C_{2v}$ | 229 | Minimum |
| $2\,^2A_1$ upper ($2\,^2E'$) | $5.170, 4.206, 5.170$ ($3.067, 2.103, 3.067$) | $C_{2v}$ | 686 | First-order saddle point imag. freq. asymmetric stretch mode |
| $2\,^2B_1$ ($2\,^2E'$) | $4.825, 4.825, 4.825$ ($2.413, 2.413, 2.413$) | $D_{3h}$ | 1165 | First-order saddle point imag. freq. symmetric stretch mode |
| $3\,^2A_1$ ($1\,^2A_1'$) | $4.557, 4.557, 4.557$ ($2.279, 2.279, 2.279$) | $D_{3h}$ | 1898 | Minimum |
| $1\,^2A_2$ ($1\,^2E''$) | $4.337, 5.132, 4.337$ ($1.771, 2.566, 2.566$) | $C_{2v}$ | 4286 | Minimum |
| $2\,^2B_2$ ($1\,^2E''$) | $4.742, 4.208, 4.742$ ($2.638, 2.104, 2.104$) | $C_{2v}$ | 4366 | First-order saddle point imag. freq. asymmetric stretch mode |
| $4\,^2A_1$ lower ($2\,^2A_1'$) | $4.603, 5.414, 4.603$ ($1.896, 2.707, 2.707$) | $C_{2v}$ | 5431 | Local $C_{2v}$ extremum, true classification failed |
| $4\,^2A_1$ upper ($2\,^2A_1'$) | $5.138, 4.350, 5.138$ ($2.963, 2.175, 2.175$) | $C_{2v}$ | 5446 | Local $C_{2v}$ extremum, true classification failed |
| $3\,^2B_1$ ($3\,^2E'$) | $4.921, 4.893, 4.921$ ($2.475, 2.447, 2.447$) | $C_{2v}$ | 6097 | Local $C_{2v}$ extremum, true classification failed |
| $4\,^2B_1$ ($1\,^2A_2'$) | $5.215, 5.215, 5.215$ ($2.608, 2.608, 2.608$) | $D_{3h}$ | 7077 | Local $C_{2v}$ extremum, true classification failed |
| $1\,^1A_1$ ($^1A_1'$) | $4.610, 4.610, 4.610$ ($2.305, 2.305, 2.305$) | $D_{3h}$ | 19942 | Minimum |

Table S.IV. Synopsis of **linear** ($D_{\infty h}$) doublet and quartet (ground and excited) states of $Rb_3$ as well as the triplet state of $Rb_3{}^+$ computed at MRCI(ECP+CPP)/UET15 level of theory.

| State ($D_{\infty h}$) | $R_{12}, R_{23}, R_{13}$ [Å] ($R_1, R_2, R_3$) | $E_{\mathrm{rel}}$ [cm$^{-1}$] | Classification |
|---|---|---|---|
| $1\,{}^4\mathrm{B}_1$ ($1\,{}^4\Sigma_u^+$) | $5.916, 11.831, 5.916$ $(0.000, 5.916, 5.916)$ | -551 | First-order saddle point |
| $1\,{}^4\mathrm{A}_2 + 2\,{}^4\mathrm{B}_1$ ($1\,{}^4\Pi_g$) | $4.435, 8.869, 4.435$ $(0.000, 4.435, 4.435)$ | 4044 | Renner-Teller pair with $2\,{}^4\mathrm{B}_1$ turning out as saddle point |
| $1\,{}^4\mathrm{A}_1 + 1\,{}^4\mathrm{B}_2$ ($1\,{}^4\Pi_u$) | $4.581, 9.162, 4.581$ $(0.000, 4.581, 4.581)$ | 7180 | Both first-order saddle points due to PJT interaction with $2\,{}^4\mathrm{A}_1$ |
| $1\,{}^4\mathrm{A}_1$ ($1\,{}^4\Pi_u \to 1\,{}^4\Sigma_g^+$) | $5.248, 10.495, 5.248$ $(0.000, 5.248, 5.248)$ | 7289 | First-order saddle point |
| $2\,{}^4\mathrm{A}_1$ ($1\,{}^4\Sigma_g^+ \to 1\,{}^4\Pi_u$)[a] | $4.937, 9.874, 4.937$ $(0.000, 4.937, 4.937)$ | 7442 | Minimum |
| $3\,{}^4\mathrm{B}_1$ ($2\,{}^4\Sigma_u^+$) | $4.660, 9.319, 4.660$ $(0.000, 4.660, 4.660)$ | 10924 | First-order saddle point |
| $1\,{}^2\mathrm{B}_1$ ($1\,{}^2\Sigma_u^+$) | $4.357, 8.714, 4.357$ $(0.000, 4.357, 4.357)$ | -5396 | First-order saddle point |
| $1\,{}^2\mathrm{A}_1$ ($1\,{}^2\Sigma_g^+$) | $4.795, 9.590, 4.795$ $(0.000, 4.795, 4.795)$ | -2109 | Minimum |
| $2\,{}^2\mathrm{A}_1$ ($1\,{}^2\Pi_u \to 2\,{}^2\Sigma_g^+$)[a] | $4.755, 9.510, 4.755$ $(0.000, 4.755, 4.755)$ | 3135 | First-order saddle point |
| $2\,{}^2\mathrm{A}_1 + 1\,{}^2\mathrm{B}_2$ ($1\,{}^2\Pi_u$) | $4.213, 8.426, 4.213$ $(0.000, 4.213, 4.213)$ | 3243 | True classification failed |
| $3\,{}^2\mathrm{A}_1$ ($2\,{}^2\Sigma_g^+ \to 1\,{}^2\Pi_u$)[a] | $4.440, 8.880, 4.440$ $(0.000, 4.440, 4.440)$ | 3390 | Minimum |
| $1\,{}^2\mathrm{A}_2 + 2\,{}^2\mathrm{B}_1$ ($1\,{}^2\Pi_g$) | $4.358, 8.716, 4.358$ $(0.000, 4.358, 4.358)$ | 4939 | $2\,{}^2\mathrm{B}_1$ first-order saddle point, $1\,{}^2\mathrm{A}_2$ classification failed |
| $2\,{}^2\mathrm{B}_1$ ($1\,{}^2\Pi_g \to 2\,{}^2\Sigma_u^+$)[a] | $5.014, 10.028, 5.014$ $(0.000.5.014, 5.014)$ | 5634 | First-order saddle point |
| $3\,{}^2\mathrm{B}_1$ ($2\,{}^2\Sigma_u^+ \to 1\,{}^2\Pi_g$)[a] | $4.930, 9.860, 4.930$ $(0.000, 4.930, 4.930)$ | 5647 | Minimum |
| $4\,{}^2\mathrm{B}_1$ ($3\,{}^2\Sigma_u^+$) | $4.961, 9.922, 4.961$ $(0.000, 4.961, 4.961)$ | 7664 | First-order saddle point |
| $4\,{}^2\mathrm{A}_1$ ($3\,{}^2\Sigma_g^+$) | $5.197, 10.394, 5.197$ $(0.000, 5.197, 5.197)$ | 8221 | True classification failed |
| $1\,{}^3\mathrm{B}_1$ (${}^3\Sigma_u^+$) | $4.875, 9.749, 4.875$ $(0.000, 4.875, 4.875)$ | 24043 | Minimum |

[a] Consequence of a combined pseudo Jahn-Teller and Renner-Teller interaction where two $\mathrm{A}_1$ ($\mathrm{B}_1$) states interchange scanning along $D_{\infty h}$ geometries. Hence non-degenerate frequencies $\tilde{\nu}_{\mathrm{bending}_{1,2}}$

## SYMMETRY-INDUCED COUPLING EFFECTS – DEGENERATE STATES AND VIBRONIC COUPLING

### The (pseudo) Jahn-Teller effect

In the main text we already pointed out that homonuclear alkali-metal triatomic molecules are prominent systems showing Jahn-Teller distortions [S10, S11]. For equilateral triangular configurations, $X_3$–type molecules are also the simplest systems with a 3–fold axis of symmetry ($D_{3h}$ point group symmetry) allowing for 2–fold degenerate E terms in ground or excited states, cf. the corresponding character table in Tab. S.VIII. If the equilateral triangle is distorted, the E term splits leaving a conical intersection (COIN) on the (adiabatic) potential energy surface (APES) at the high-symmetry point of degeneracy. This is known as the *Jahn-Teller (JT) effect* where the JT theorem further states that highly symmetric non-linear geometries in degenerate electronic states are not stable equilibrium configurations, with the system lowering its symmetry. This kind of vibronic coupling in $X_3$ systems is called the $\mathrm{E} \otimes \mathrm{e}$ JT effect describing the interaction of a two-fold degenerate electronic E term with a twofold degenerate e vibration. The main effect of electronic degeneracy is that it produces a special coupling between the electronic and nuclear motion. This leads to a series of observable effects, which are jointly called the JT vibronic coupling effects. For in-depth information on the JT effect theory see, e.g., Ref. [S12].

In addition to the JT effect, the vibronic mixing of two (or several) nearly degenerate electronic states under nuclear displacements, i.e. the so called *pseudo Jahn-Teller (PJT) effect*, also plays a crucial role in the structural instability of high-symmetry configurations [S11]. In $X_3$-type systems cases where E and A states (according to $D_{3h}$ IRREPs) which are close in energy can emerge are of particular interest. For more details on PJT theory see, e.g., Ref. [S13].

In order to study the main topological features of the PESs of $Rb_3$ coming with the (P)JT effect we introduced (symmetry-adapted) JT normal coordinates $Q_1$, $Q_2$ and $Q_3$ describing the planar vibrational modes of systems in $D_{3h}$ symmetry (breathing mode, fully asymmetric and symmetric stretch mode, respectively) [S11]. Referring to Ref. [S2, S14–S16] we perform one-dimensional scans along the $Q_3$ mode (thus retaining $C_{2v}$ symmetry). In general this can be done by varying $Q_3$ while keeping $Q_1$ fixed to the value, e.g., corresponding to the ground state geometry and setting $Q_2 = 0$. We present our results in Figs. S3. The energies of the depicted adiabatic potential energy curves (APECs) are also given with respect to the free atom-atom-atom limit (i.e. $3 \cdot 5s$-asymptote) and the states are labeled

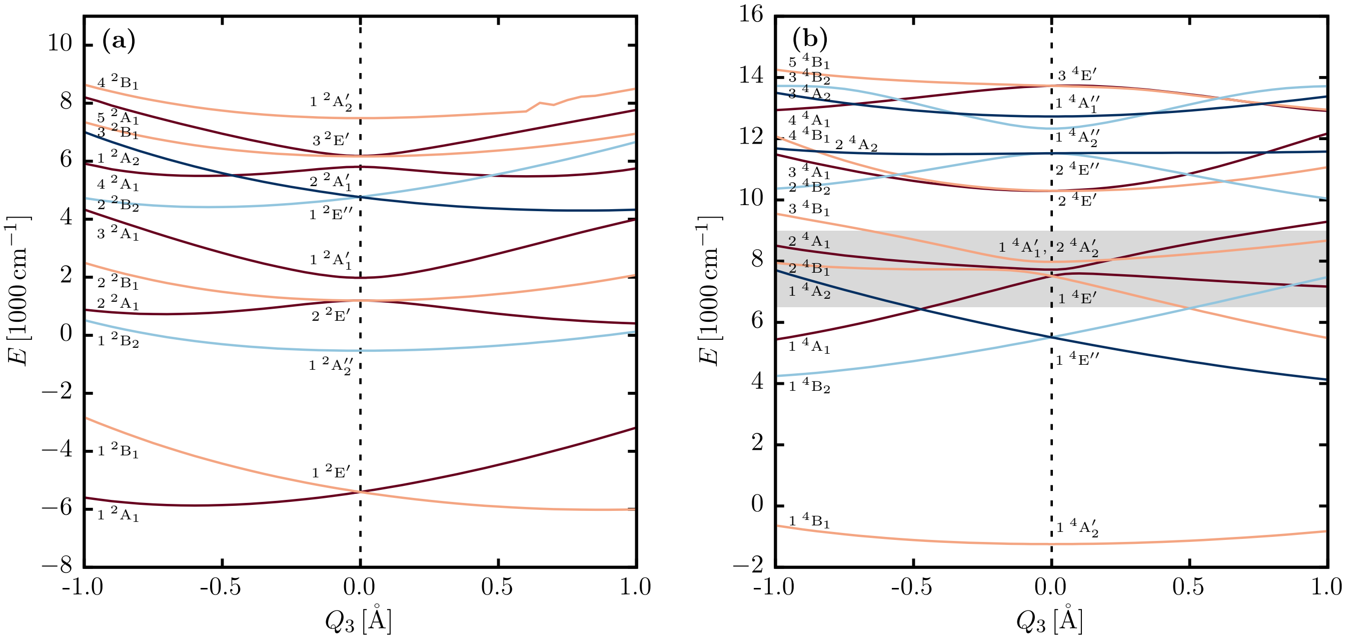


Figure S3. Adiabatic potential energy curves (APECs) for the **doublet states** in **(a)** of $Rb_3$ scanned along the symmetric stretching mode $Q_3$ with $Q_1 = 8.1701$ Å and $Q_2 = 0.0$ Å maintaining $C_{2v}$ symmetry. **Quartet states** are shown in **(b)** with $Q_1 = 9.1989$ Å and $Q_2 = 0.0$ Å. The curves are labeled according to the irreducible representations of the point group $C_{2v}$ with the respective labels ($D_{3h}$ IRREPS) for equilateral triangular configurations at $Q_3 = 0.0$ Å. The area highlighted in gray represents a submanifold ($\mathcal{Q}$ in the main text) of excited quartet states where a complicated interplay between avoided crossings, conical intersections and JT interactions is present.

Table S.V. Overview on (pseudo) Jahn-Teller (P)JT pairs for the doublet and quartet states listed in Tab. S.III. For equilateral triangular configurations (i.e. $D_{3h}$ symmetry) we obtain degeneracies forming a one-dimensional conical intersection (COIN) seam in the three-dimensional configuration space. Listed are the lowest COINs, i.e. the minima of the one-dimensional APECs in $D_{3h}$ symmetry, their branching states w.r.t. to symmetry-lowering $C_{2v}$ distortions and the corresponding classification if also PJT interactions are present.

| State ($D_{3h}$) | Components ($C_{2v}$) | $R_{12}, R_{23}, R_{13}$ [Å] ($R_1, R_2, R_3$) | Lowest COIN ($D_{3h}$ PEC minimum) [cm$^{-1}$] | Classification |
|---|---|---|---|---|
| $1\,^4$E$'$ | $1\,^4$A$_1$ + $2\,^4$B$_1$ | 4.879, 4.879, 4.879 (2.440, 2.440, 2.440) | 7202 | JT pair but part of $\mathcal{Q}$ manifold |
| $2\,^4$E$'$ | $3\,^4$A$_1$ + $4\,^4$B$_1$ | 5.305, 5.305, 5.305 (2.653, 2.653, 2.653) | 10302 | JT pair |
| $3\,^4$E$'$ | $4\,^4$A$_1$ + $5\,^4$B$_1$ | 5.148, 5.148, 5.148 (2.574, 2.574, 2.574) | 13707 | JT pair |
| $1\,^4$E$''$ | $1\,^4$B$_2$ + $1\,^4$A$_2$ | 4.500, 4.500, 4.500 (2.250, 2.250, 2.250) | 4146 | JT pair |
| $2\,^4$E$''$ | $2\,^4$B$_2$ + $2\,^4$A$_2$ | 4.916, 4.916, 4.916 (2.458, 2.458, 2.458) | 11271 | Possibly PJT with $3\,^4$A$_2$ or $3\,^4$B$_2$ |
| $1\,^2$E$'$ | $1\,^2$A$_1$ + $1\,^2$B$_1$ | 4.546, 4.546, 4.546 (2.273, 2.273, 2.273) | -5494 | JT pair |
| $2\,^2$E$'$ | $2\,^2$A$_1$ + $2\,^2$B$_1$ | 4.824, 4.824, 4.824 (2.412, 2.412, 2.412) | 1167 | PJT with $3\,^2$A$_1$ |
| $3\,^2$E$'$ | $5\,^2$A$_1$ + $3\,^2$B$_1$ | | | PJT with $4\,^2$A$_1$ |
| $1\,^2$E$''$ | $2\,^2$B$_2$ + $1\,^2$A$_2$ | 4.500, 4.500, 4.500 (2.250, 2.250, 2.250) | 4624 | JT pair |

according to their corresponding IRREP of the $C_{2v}$ point group.

A special situation is given in the area highlighted in gray in Fig. S3 which corresponds to the manifold $\mathcal{Q}$ described in the main text. Here it appears that the four states show quadruply interactions among each others.

$$\mathcal{Q} = \{1\,^4\mathrm{A}_1, 2\,^4\mathrm{B}_1, 2\,^4\mathrm{A}_1, 3\,^4\mathrm{B}_1\}\,. \tag{S5}$$

In Tab. S.V we provide a summary of present JT and PJT couplings for both doublet and quartet states of $Rb_3$. For each equilateral triangular configuration JT pairs form a COIN. Thus, with respect to the full three dimensional configuration space, we obtain a one-dimensional COIN seam for which we can extract the corresponding minimum energies. This helps us to define a stabilization energy of the actual minimum of a JT state, cf. Ref. [S10].

## Stabilization and Localization Energy of the $1\,^4$E$''$ Jahn-Teller pair

In Jahn-Teller effect theory it is convenient [S10] to define a stabilization energy as well as a localization energy on the $E_-$ PES of a given JT pair. In the main text the stabilization energy is defined for the cut through the $1\,^4$A$_2$ minimum and is $E_s[\min(1\,^4\mathrm{A}_2)] = 991\,\mathrm{cm}^{-1}$. However, it is also possible to define it relative to the energetically lowest COIN where it takes a value of $E_s[\min(\mathrm{COIN})] = 749\,\mathrm{cm}^{-1}$. The localization energy defines the barrier height between the three equivalent minima in the tricorn potential $E_-$ depicted in the lower inset of Fig. 8 **(a)** in the main text. Figure S4 illustrates how these quantities are defined.

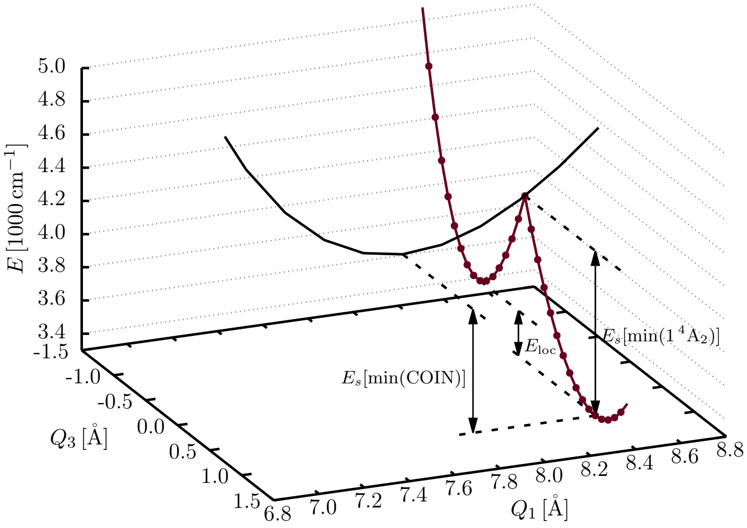


Figure S4. Cut through the $E_-$ PES of the 1 $^4$E$''$ Jahn-Teller (JT) pair for $Q_1 = 8.335$ Å, the position of the 1 $^4$A$_2$ minimum (dark red). The black line represents the one-dimensional conical intersection seam. Compare Fig. 8 **(b)** of the main text. In JT effect theory it is convenient to define a stabilization energy $E_s$ as well as a localization energy $E_{\text{loc}}$. The visual clarification of these quantities is shown here.

### Addition: Interactions in the Vicinity of the 1 $^4$E$''$ Global Minimum

Figure S5 illustrates the intersection pattern of the 1 $^4$A$_2$ state with both quartet and doublet states in close proximity to its global minimum. Here, the spin-orbit coupling (SOC) between the 1 $^4$A$_2$ and 3 $^2$A$_1$ states is in the order of 20 cm$^{-1}$. However, in this vicinity strongest SOCs of the 1 $^4$A$_2$ state are to the quartet ground state 1 $^4$B$_1$ and the 1 $^4$A$_1$ state (cf. main text). Therefore we do not expect difficulties despite the close intersection of the 3 $^2$A$_1$ state to the 1 $^4$A$_2$ global minimum.

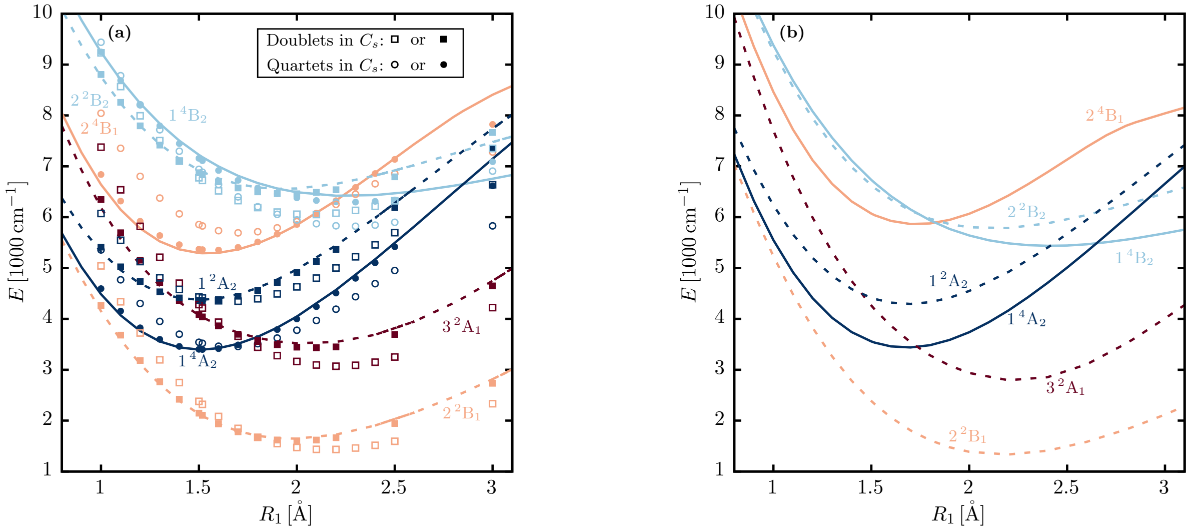


Figure S5. One-dimensional scans along the perimetric coordinate $R_1$ for different arrangements of $R_2$ and $R_3$ to study intersections in close proximity to the 1 $^4$A$_2$ global minimum. **(a)** Solid and dashed lines represent quartet and doublet states, respectively, with $R_2 = R_3 = 2.85$ Å (i.e. $C_{2v}$ scans with the 1 $^4$A$_2$ global minimum at $R_1 = 1.518$ Å, cf. Tab. S.III). Circles and squares correspond to quartet and doublet states, respectively, which are slightly distorted to $C_s$ geometries. Filled symbols represent configurations with $R_2 = 2.85$ Å and $R_3 = 2.8$ Å while open symbols correspond to $R_2 = 2.85$ Å and $R_3 = 2.55$ Å. **(b)** Solid and dashed lines represent quartet and doublet states, respectively, with $R_2 = R_3 = 2.65$ Å.

**Coupling effects for linear configurations**

In Fig. S6 we provide an overview of states when varying $R_{23}$ in an one-dimensional scan while adjusting the molecular geometry to linear configurations according to Fig. S1. We obtain doubly degenerate states forming $\Pi$ states (according to the $D_{\infty h}$ IRREP). As the states are labelled according to the $C_{2v}$ IRREPs we can extract the components belonging to the respective degenerate pairs resulting in the following $\Pi$ states. In case of the doublet spin multiplicity we obtain

$$1\,^2\Pi_u = 2\,^2\mathrm{A}_1 + 1\,^2\mathrm{B}_2\,, \tag{S6a}$$

$$1\,^2\Pi_g = 2\,^2\mathrm{B}_1 + 1\,^2\mathrm{A}_2\,, \tag{S6b}$$

$$2\,^2\Pi_u = 5\,^2\mathrm{A}_1 + 2\,^2\mathrm{B}_2\,. \tag{S6c}$$

For the quartet spin multiplicity we obtain

$$1\,^4\Pi_g = 2\,^4\mathrm{B}_1 + 1\,^4\mathrm{A}_2\,, \tag{S7a}$$

$$1\,^4\Pi_u = 1\,^4\mathrm{A}_1 + 1\,^4\mathrm{B}_2\,, \tag{S7b}$$

$$2\,^4\Pi_u = 3\,^4\mathrm{A}_1 + 2\,^4\mathrm{B}_2\,. \tag{S7c}$$

In Ref. [S17] it has been shown that for linear molecules in degenerate states the RTE is not the only (and not even the main) source of bending instability; the pseudo Jahn-Teller effect (PJTE) is most important for bending. This means that for states which are close in energy the main reason for the symmetry distortion is, in many cases, due to the PJTE, or a combined PJT plus RT interaction, rather than solely the RTE. For homonuclear triatomics relatively close-in-energy $\Pi$ and $\Sigma$ states are of particular interest. As a consequence of this combined PJT and RT interaction two $\mathrm{A}_1$ states, one of them arising from a $\Pi_u$ state can mix for greater displacements along $D_{\infty h}$ geometries. This can be also seen in Fig. S6. For instance this is the case for the $1\,^4\mathrm{A}_1$, $1\,^4\mathrm{B}_2$ states and the $2\,^4\mathrm{A}_1$ state (the PJTE counterpart).

When lowering the symmetry to, e.g., $C_{2v}$ configurations the degeneracy is lifted. To visualize this splitting of degenerate states of linear molecules when lowering the symmetry it is convenient to introduce a bending coordinate. Given the isosceles triangular configuration in Fig. S1 we define this coordinate via

$$\tilde{\varrho} = \sqrt{R_{12}^2 - (R_{23}/2)^2}\,, \tag{S8}$$

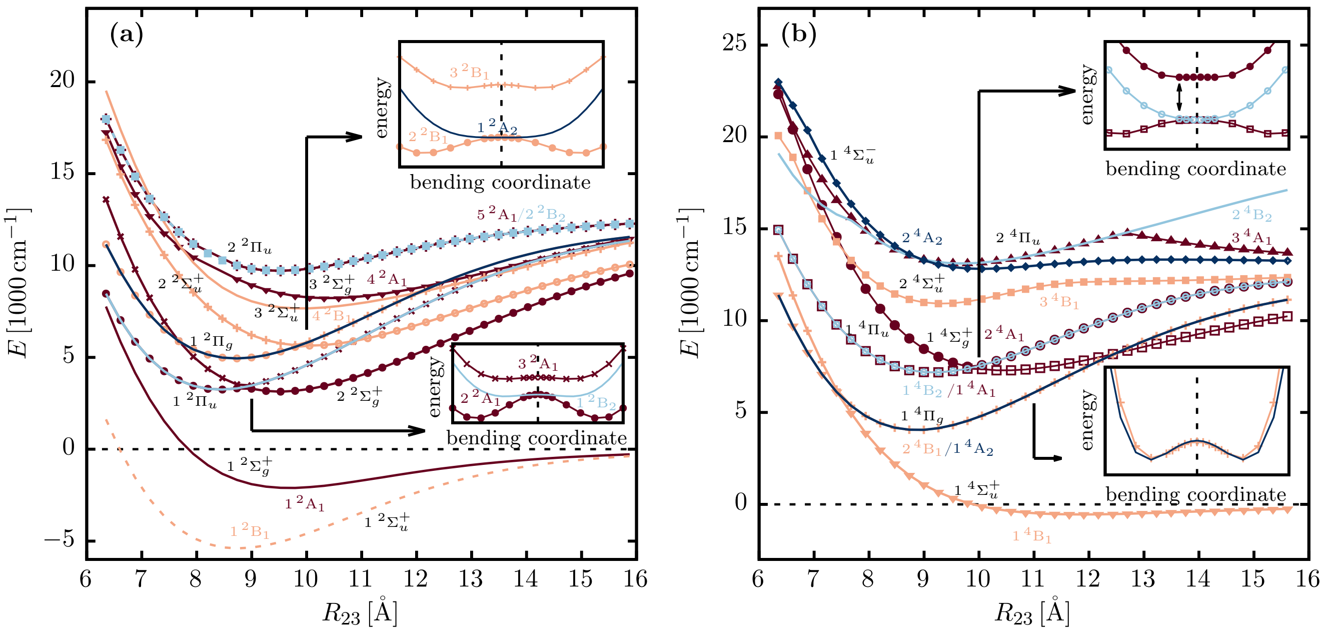


Figure S6. One-dimensional cuts along the high-symmetry $D_{\infty h}$ subspace for doublets in **(a)** and quartets in the **(b)**.

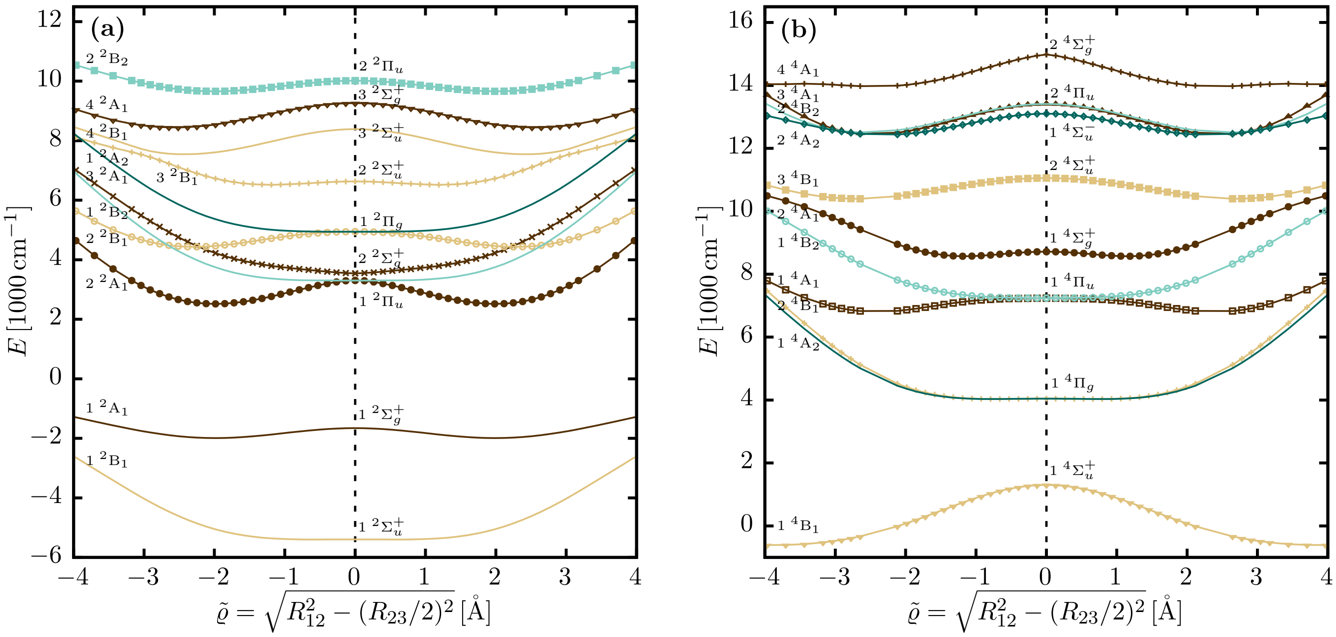


Figure S7. One-dimensional cuts of the PESs along the bending coordinate $\tilde{\varrho}$ defined in Eq. (S8) representing insertion scans from $C_{2v}$ configurations to linear $D_{\infty h}$ to the inverted $C_{2v}$ structure, for both doublet and quartet states of $Rb_3$. **(a)** Doublet states of $Rb_3$ for a fixed value of $R_{23} = 8.714$ Å, the $D_{\infty h}$ extremum of the 1 $^2B_1$ state. **(b)** Insertion scan for the quartet states of $Rb_3$ keeping $R_{23} = 8.869$ Å fixed (value for the $D_{\infty h}$ minimum of the 2 $^4B_1$/1 $^4A_2$ states).

with fixed bond distance $R_{23}$. When scanning along $\tilde{\varrho}$ this can be viewed as an insertion scan $C_{2v} \to D_{\infty h} \to C_{2v}$. The result is depicted in Fig. S7.

## SELECTION RULES AND GROUP THEORY

### Selection Rules for $C_{2v}$ configurations

To deduce the selection rules using group theoretical arguments we use the character- and multiplication tables of the respective point group. For in-depth information on group theory see, e.g., Ref. [S18]. The $C_{2v}$ point group consists of four irreducible representations (IRREPs) $\mathrm{A}_1$, $\mathrm{A}_2$, $\mathrm{B}_1$, $\mathrm{B}_2$ and is defined by the symmetry operations $E$ (identity operator), $C_2$ (twofold rotation axis with respect to a chosen preferential direction, here $z$) and the two mirror planes $\sigma_v(xz)$ and $\sigma_d(yz)$ (choice of $xz$ and $yz$ plane by convention). The corresponding character table is given in Tab. S.VI, with the multiplication table defining the direct product between two IRREPs given in Tab. S.VII. Since

Table S.VI. Character table for the $C_{2v}$ point group.

| | $E$ | $C_2(z)$ | $\sigma_v(xz)$ | $\sigma_d(yz)$ | linear functions, rotations | quadratic functions |
|---|---|---|---|---|---|---|
| $\mathrm{A}_1$ | +1 | +1 | +1 | +1 | $z$ | $x^2$, $y^2$, $z^2$ |
| $\mathrm{A}_2$ | +1 | +1 | −1 | −1 | $R_z$ | $xy$ |
| $\mathrm{B}_1$ | +1 | −1 | +1 | −1 | $x$, $R_y$ | $xz$ |
| $\mathrm{B}_2$ | +1 | −1 | −1 | +1 | $y$, $R_x$ | $yz$ |

Table S.VII. Multiplication table of the $C_{2v}$ point group for building direct products between the different IRREPs, e.g. $\mathrm{B}_1 \otimes \mathrm{A}_2 = \mathrm{B}_2$.

| | $\mathrm{A}_1$ | $\mathrm{A}_2$ | $\mathrm{B}_1$ | $\mathrm{B}_2$ |
|---|---|---|---|---|
| $\mathrm{A}_1$ | $\mathrm{A}_1$ | $\mathrm{A}_2$ | $\mathrm{B}_1$ | $\mathrm{B}_2$ |
| $\mathrm{A}_2$ | $\mathrm{A}_2$ | $\mathrm{A}_1$ | $\mathrm{B}_2$ | $\mathrm{B}_1$ |
| $\mathrm{B}_1$ | $\mathrm{B}_1$ | $\mathrm{B}_2$ | $\mathrm{A}_1$ | $\mathrm{A}_2$ |
| $\mathrm{B}_2$ | $\mathrm{B}_2$ | $\mathrm{B}_1$ | $\mathrm{A}_2$ | $\mathrm{A}_1$ |

vector spaces can be also constructed from functions it is convenient to consider the transformation properties of some functions with respect to the symmetry operations of the point group as well. This is what is listed in the last two columns of Tab. S.VI. The functions here are chosen to help when dealing with quantum chemical problems like the dipole operator ($\propto \vec{r}$) and orbitals or rotations $R_i$ with respect to a given axis $i \in \{x, y, z\}$.

As described above wavefunctions of different symmetry do not mix and their corresponding PESs can intersect. Thus, the first criterion for mixing or coupling of states is defined by their corresponding configuration. Another possibility for mixing of states is given by non-vanishing electronic dipole transition moments. Since we are labeling states according to the IRREPs of the point group $C_{2v}$ let us investigate selection rules for finite electronic dipole transition moments. First of all the total spin of initial and final states must be the same, i.e.

$$\Delta S = 0\,. \tag{S9}$$

Given the dipole operator

$$\hat{\mu} = -q\hat{\mathbf{r}}\,, \tag{S10}$$

with the charge $q$ and the position operator $\hat{\mathbf{r}} = (\hat{x}, \hat{y}, \hat{z})^T$, non-vanishing transitions obey the *necessary* condition

$$\langle i|\hat{\mu}|f\rangle \neq 0 \quad \Longrightarrow \quad \Gamma(|i\rangle) \otimes \Gamma(\hat{\mu}) \otimes \Gamma(|f\rangle) = \mathrm{A}_1\,. \tag{S11}$$

This is, the direct product of the corresponding IRREPs $\Gamma^{(i)}$ must yield the totally symmetric IRREP $\mathrm{A}_1$ (in terms of the point group $C_{2v}$). Using Tab. S.VI to identify the corresponding IRREPs of the components of the dipole operator $\hat{\mu}_i\,, i \in \{x, y, z\}$, we obtain the following couplings which can be $\neq 0$

$$\hat{\mu}_x : \quad \langle \mathrm{A}_1\,|\,\hat{\mu}_x\,|\,\mathrm{B}_1\rangle\ ,\ \langle \mathrm{B}_2\,|\,\hat{\mu}_x\,|\,\mathrm{A}_2\rangle\ , \tag{S12}$$

and

$$\hat{\mu}_y : \quad \langle \mathrm{A}_1\,|\,\hat{\mu}_y\,|\,\mathrm{B}_2\rangle\ ,\ \langle \mathrm{B}_1\,|\,\hat{\mu}_y\,|\,\mathrm{A}_2\rangle\ , \tag{S13}$$

and

$$\hat{\mu}_z: \quad \langle \mathrm{A}_1 \,|\, \hat{\mu}_z \,|\, \mathrm{A}_1 \rangle \;, \langle \mathrm{B}_1 \,|\, \hat{\mu}_z \,|\, \mathrm{B}_1 \rangle \;, \langle \mathrm{B}_2 \,|\, \hat{\mu}_z \,|\, \mathrm{B}_2 \rangle \;, \langle \mathrm{A}_2 \,|\, \hat{\mu}_z \,|\, \mathrm{A}_2 \rangle \;. \tag{S14}$$

With this only quartet-quartet- or doublet-doublet-couplings, respectively, are possible.

Additionally considering *spin-orbit coupling* effects we note that also couplings with

$$\Delta S = 0, \pm 1 \tag{S15}$$

become possible allowing for doublet-quartet mixing and vice versa. Using the same approach as before (i.e. the direct product of initial state, spin-orbit operator and final state should yield the totally symmetric IRREP $\mathrm{A}_1$) we can easily convince ourselves (using Tabs. S.VI and S.VII) that the following mixings induced by the spin-orbit operator can be $\neq 0$

$$(\hat{\mathbf{L}}\hat{\mathbf{S}})_x: \qquad \left\langle \mathrm{A}_1 \middle| (\hat{\mathbf{L}}\hat{\mathbf{S}})_x \middle| \mathrm{B}_2 \right\rangle \,, \left\langle \mathrm{B}_1 \middle| (\hat{\mathbf{L}}\hat{\mathbf{S}})_x \middle| \mathrm{A}_2 \right\rangle \,, \tag{S16}$$

and

$$(\hat{\mathbf{L}}\hat{\mathbf{S}})_y: \qquad \left\langle \mathrm{A}_1 \middle| (\hat{\mathbf{L}}\hat{\mathbf{S}})_y \middle| \mathrm{B}_1 \right\rangle \,, \left\langle \mathrm{B}_2 \middle| (\hat{\mathbf{L}}\hat{\mathbf{S}})_y \middle| \mathrm{A}_2 \right\rangle \,, \tag{S17}$$

and

$$(\hat{\mathbf{L}}\hat{\mathbf{S}})_z: \qquad \left\langle \mathrm{B}_1 \middle| (\hat{\mathbf{L}}\hat{\mathbf{S}})_z \middle| \mathrm{B}_2 \right\rangle \,, \left\langle \mathrm{A}_1 \middle| (\hat{\mathbf{L}}\hat{\mathbf{S}})_z \middle| \mathrm{A}_2 \right\rangle \,. \tag{S18}$$

*Note:* Again, since Eq. (S15) is valid in this case we obtain quartet-quartet, doublet-doublet as well as doublet-quartet mixing.

### Selection Rules for $D_{3h}$ configurations

To deduce the selection rules for $D_{3h}$ configurations using group theoretical arguments, again we first need the corresponding character- and multiplication tables of the $D_{3h}$ point group. This group has six IRREPs where Tab. S.VIII shows their corresponding behaviour with respect to the respective symmetry operations. The group contains the symmetry operations $E$ (i.e. the identity), the rotation axis $C_3$ (where $2C_3$ indicates that the rotation is either clockwise or counter-clockwise), three $C_2$ rotation axes, one horizontal mirror plane $\sigma_h$, three vertical mirror planes $\sigma_v$ and the rotation-reflection around the alternating axis $S_3$ (where $2S_3$ again indicates that there is also the inverse operation). Again, the last two columns give the transformation properties of given functions with respect to the corresponding symmetry operations of the point group. The multiplication table defining the direct products

Table S.VIII. Character table for the $D_{3h}$ point group.

| | $E$ | $2C_3$ | $3C_2$ | $\sigma_h$ | $2S_3$ | $3\sigma_v$ | lin. funct., rot. | quad. funct. |
|---|---|---|---|---|---|---|---|---|
| $\mathrm{A}_1'$ | 1 | 1 | 1 | 1 | 1 | 1 | – | $x^2+y^2$, $z^2$ |
| $\mathrm{A}_2'$ | 1 | 1 | −1 | 1 | 1 | −1 | $R_z$ | – |
| $\mathrm{E}'$ | 2 | −1 | 0 | 2 | −1 | 0 | $x$, $y$ | $x^2-y^2$, $2xy$ |
| $\mathrm{A}_1''$ | 1 | 1 | 1 | −1 | −1 | −1 | – | – |
| $\mathrm{A}_2''$ | 1 | 1 | −1 | −1 | −1 | 1 | $z$ | – |
| $\mathrm{E}''$ | 2 | −1 | 0 | −2 | 1 | 0 | $R_x$, $R_y$ | $xy$, $yz$ |

between any two IRREPs is given in Tab. S.IX.

Let us also consider the corresponding selection rules in case of $D_{3h}$ configurations, i.e. for equilateral triangles. At this the necessary condition from Eq. (S11) reads

$$\langle i|\hat{\mu}|f\rangle \neq 0 \qquad \Longrightarrow \qquad \Gamma(|i\rangle) \otimes \Gamma(\hat{\mu}) \otimes \Gamma(|f\rangle) = \mathrm{A}_1' \,. \tag{S19}$$

Using Tabs. S.VIII and S.IX to deduce the selection rules we obtain the following electronic tranistion dipole elements which can be $\neq 0$

$$\begin{aligned} \hat{\mu}_{x,y}: \quad & \langle \mathrm{A}_1' \,|\, \hat{\mu}_{x,y} \,|\, \mathrm{E}' \rangle \;, \langle \mathrm{A}_2' \,|\, \hat{\mu}_{x,y} \,|\, \mathrm{E}' \rangle \;, \langle \mathrm{E}' \,|\, \hat{\mu}_{x,y} \,|\, \mathrm{E}' \rangle \;, \\ & \langle \mathrm{A}_1'' \,|\, \hat{\mu}_{x,y} \,|\, \mathrm{E}'' \rangle \;, \langle \mathrm{A}_2'' \,|\, \hat{\mu}_{x,y} \,|\, \mathrm{E}'' \rangle \;, \langle \mathrm{E}'' \,|\, \hat{\mu}_{x,y} \,|\, \mathrm{E}'' \rangle \;, \end{aligned} \tag{S20}$$

Table S.IX. Multiplication table for the $D_{3h}$ point group.

| | $A'_1$ | $A'_2$ | $E'$ | $A''_1$ | $A''_2$ | $E''$ |
|---|---|---|---|---|---|---|
| $A'_1$ | $A'_1$ | $A'_2$ | $E'$ | $A''_1$ | $A''_2$ | $E''$ |
| $A'_2$ | $A'_2$ | $A'_1$ | $E'$ | $A''_2$ | $A''_1$ | $E''$ |
| $E'$ | $E'$ | $E'$ | $A'_1 + A'_2 + E'$ | $E''$ | $E''$ | $A''_1 + A''_2 + E''$ |
| $A''_1$ | $A''_1$ | $A''_2$ | $E''$ | $A'_1$ | $A'_2$ | $E'$ |
| $A''_2$ | $A''_2$ | $A''_1$ | $E''$ | $A'_2$ | $A'_1$ | $E'$ |
| $E''$ | $E''$ | $E''$ | $A''_1 + A''_2 + E''$ | $E'$ | $E'$ | $A'_1 + A'_2 + E'$ |

and

$$\hat{\mu}_z : \quad \langle A'_1 \,|\, \hat{\mu}_z \,|\, A''_2 \rangle \;,\; \langle A'_2 \,|\, \hat{\mu}_z \,|\, A''_1 \rangle \;,\; \langle E' \,|\, \hat{\mu}_z \,|\, E'' \rangle \;. \tag{S21}$$

Using the same approach we can also deduce the selection rules due to spin-orbit coupling for $D_{3h}$ configurations. Again, applying Tabs. S.VIII and S.IX we obtain that the following matrix elements can be $\neq 0$

$$\begin{aligned}(\hat{\mathbf{L}}\hat{\mathbf{S}})_{x,y} : \qquad & \left\langle A'_1 \middle| (\hat{\mathbf{L}}\hat{\mathbf{S}})_{x,y} \middle| E'' \right\rangle ,\; \left\langle A'_2 \middle| (\hat{\mathbf{L}}\hat{\mathbf{S}})_{x,y} \middle| E'' \right\rangle ,\; \left\langle A''_1 \middle| (\hat{\mathbf{L}}\hat{\mathbf{S}})_{x,y} \middle| E' \right\rangle , \\ & \left\langle A''_2 \middle| (\hat{\mathbf{L}}\hat{\mathbf{S}})_{x,y} \middle| E' \right\rangle ,\; \left\langle E' \middle| (\hat{\mathbf{L}}\hat{\mathbf{S}})_{x,y} \middle| E'' \right\rangle ,\end{aligned} \tag{S22}$$

and

$$(\hat{\mathbf{L}}\hat{\mathbf{S}})_z : \qquad \left\langle A'_1 \middle| (\hat{\mathbf{L}}\hat{\mathbf{S}})_z \middle| A'_2 \right\rangle ,\; \left\langle E' \middle| (\hat{\mathbf{L}}\hat{\mathbf{S}})_z \middle| E' \right\rangle ,\; \left\langle A''_1 \middle| (\hat{\mathbf{L}}\hat{\mathbf{S}})_z \middle| A''_2 \right\rangle ,\; \left\langle E'' \middle| (\hat{\mathbf{L}}\hat{\mathbf{S}})_z \middle| E'' \right\rangle \;. \tag{S23}$$

## Subduction tables

Groups of higher order (= the number of symmetry elements) have certain subgroups, e.g. the point group $C_{2v}$ with order four is a subgroup of $D_{3h}$ with order 12. The correlation between the IRREPs of a given group and those of its subgroups is shown in so called subduction tables. In a number of cases the correlation between groups is not unique. For example in $C_s$ one has to define which plane from the parent group becomes the sole plane of $C_s$.

In this work (and in the main text) we restricted ourselves to investigations in the $C_{2v}$ subspace of possible configurations and used the corresponding IRREPs for labeling the emerging doublet and quartet states (ground and excited). As discussed, homonuclear triatomics, especially triatomic clusters of alkali metal atoms, are prominent systems showing the (P)JT and RT effects. This is, when studying the $C_{2v}$ subspace highly-symmetric configurations – namley $D_{3h}$ and $D_{\infty h}$ – are also considered. To assign the resulting high-symmetry configurations to their correct IRREP and deduce the mapping $C_{2v} \rightarrow D_{3h}$ or $C_{2v} \rightarrow D_{\infty h}$, respectively, we made use of the subduction tables in Tab. S.X and Tab. S.XI . The most general point group for investigating $X_3$ systems is $C_s$ since the three atoms always

Table S.X. Subduction $D_{3h}$ to $C_{2v}$.

| $D_{3h}$ | $C_{2v}$ $[\sigma_h \rightarrow \sigma_v(xz)]$ | $C_{2v}$ $[\sigma_h \rightarrow \sigma_v(xy)]$ | $C_{2v}$ $[\sigma_h \rightarrow \sigma_v(yz)]$ |
|---|---|---|---|
| $A_1'$ | $A_1$ | $A_1$ | $A_1$ |
| $A_2'$ | $B_1$ | $B_1$ | $B_2$ |
| $E'$ | $A_1 + B_1$ | $A_1 + B_2$ | $A_1 + B_2$ |
| $A_1''$ | $A_2$ | $A_2$ | $A_2$ |
| $A_2''$ | $B_2$ | $B_1$ | $B_1$ |
| $E''$ | $A_2 + B_2$ | $A_2 + B_1$ | $A_2 + B_1$ |

Table S.XI. Subduction $D_{\infty h}$ to $D_{2h}$ to $C_{2v}$.

| $D_{\infty h}$ | $D_{2h}$ | $C_{2v}$ $[C_2(z)]$ | $C_{2v}$ $[C_2(y)]$ | $C_{2v}$ $[C_2(x)]$ |
|---|---|---|---|---|
| $\Sigma_g^+$ | $A_g$ | $A_1$ | $A_1$ | $A_1$ |
| $\Sigma_g^-$ | $B_{1g}$ | $A_2$ | $B_2$ | $B_1$ |
| $\Sigma_u^+$ | $B_{1u}$ | $A_1$ | $B_1$ | $B_2$ |
| $\Sigma_u^-$ | $A_u$ | $A_2$ | $A_2$ | $A_2$ |
| $\Pi_g$ | $B_{2g} + B_{3g}$ | $B_1 + B_2$ | $A_2 + B_1$ | $B_2 + A_2$ |
| $\Pi_u$ | $B_{2u} + B_{3u}$ | $B_2 + B_1$ | $A_1 + B_2$ | $B_1 + A_1$ |

define a plane. When, for instance, studying the JT APES in the $Q_2$-$Q_3$ space, i.e. in the branching space where the degeneracy is lifted, we also obtain $C_s$ configurations. Therefore it is important to know the mapping $C_{2v} \rightarrow C_s$ which is shown in Tab. S.XII . As described above this correlation is not unique.

Table S.XII. Subduction table for the IRREPs from the $C_{2v}$ to the $C_s$ point group.

| $C_{2v}$ | $C_s$ $[\sigma(xz)]$ | $C_s$ $[\sigma(yz)]$ |
|---|---|---|
| $A_1$ | $A'$ | $A'$ |
| $B_1$ | $A'$ | $A''$ |
| $B_2$ | $A''$ | $A'$ |
| $A_2$ | $A''$ | $A''$ |

## OVERVIEW ON SELECTED SPIN ORBIT COUPLING EFFECTS

The following tables just serve as a first guideline to get an idea on the expected magnitude of spin-orbit coupling (SOC) effects for both doublet and quartet states of $Rb_3$.

Table S.XIII. Survey of spin-orbit coupling (SOC) effects (calculated at MRCI(ECP+CPP)/UET15 level of theory) for the previously shown extremal points (in the $C_{2v}$ subspace) of the **quartet** states of $Rb_3$ in **triangular configuration** (i.e. $D_{3h}$ or $C_{2v}$). SOC leads to a splitting into two degenerate levels (Kramers pairs). Energies are given as the difference between SO results $E$ and the corresponding unperturbed energy $E_0$

| State (geom.) | $E - E_0$ [cm$^{-1}$] | Splitting [cm$^{-1}$] | dominant couplings | strength [cm$^{-1}$] |
|---|---|---|---|---|
| $1\,^4B_1(D_{3h})$ | −0.158<br>−0.0743 | 0.0837 | $1\,^4B_2$<br>$1\,^4A_2$ | 21.35<br>14.24 |
| $1\,^4A_2(C_{2v})$ | −0.228<br>−0.618 | 0.3907 | $1\,^4A_1$<br>$1\,^4B_1$ | 30.83<br>29.95 |
| $1\,^4B_2(C_{2v})$ | 0.361<br>−0.451 | 0.8121 | $1\,^4B_1$<br>$1\,^4A_1$ | 42.82<br>21.96 |
| $2\,^4B_1(C_{2v})$ | 4.389<br>39.628 | 35.239 | $1\,^4A_2$<br>$1\,^4A_2$ | 38.58<br>44.55 |
| $1\,^4A_1(C_{2v})$ upper | −0.696<br>−3.202 | 2.506 | $2\,^4A_2$<br>$1\,^4B_2$ | 38.63<br>35.31 |
| $2\,^4A_1(D_{3h})$ | −1.819<br>−19.210 | 17.391 | $2\,^4A_2$<br>$3\,^4B_1$ | 46.17<br>48.67 |
| $3\,^4B_1(D_{3h})$ | 9.387<br>55.169 | 45.782 | $2\,^4B_2$<br>$2\,^4A_1$ | 50.64<br>52.57 |
| $2\,^4B_2(C_{2v})$ | 0.715<br>0.359 | 0.356 | $2\,^4B_1$<br>$1\,^4A_2$ | 63.54<br>26.45 |
| $4\,^4B_1(C_{2v})$ | −19.171<br>−64.433 | 45.262 | $3\,^4A_1$<br>$3\,^4A_1$ | 39.82<br>45.98 |
| $3\,^4A_1(C_{2v})$ lower | −23.718<br>−69.482 | 45.764 | $3\,^4A_2$<br>$4\,^4B_1$ | 48.29<br>46.00 |
| $2\,^4A_2(C_{2v})$ | 2.963<br>8.041 | 5.078 | $2\,^4A_1$<br>$3\,^4B_1$ | 53.33<br>32.66 |
| $3\,^4A_1(C_{2v})$ upper | −3.066<br>−0.0921 | 2.974 | $3\,^4A_2$<br>$3\,^4B_1$ | 27.68<br>20.50 |

Table S.XIV. Survey of spin-orbit coupling (SOC) effects (calculated at MRCI(ECP+CPP)/UET15 level of theory) for the previously shown extremal points (in the $C_{2v}$ subspace) of the **quartet** states of $Rb_3$in **linear configuration** (i.e. $D_{\infty h}$). SOC leads to a splitting into two degenerate levels (Kramers pairs). Energies are given as the difference between SO results $E$ and the corresponding unperturbed energy $E_0$

| State (geom.) | $E - E_0$ [cm$^{-1}$] | Splitting [cm$^{-1}$] | dominant couplings | strength [cm$^{-1}$] |
|---|---|---|---|---|
| $2\,^4B_1(D_{\infty h})$ | −76.982<br>−41.743 | 35.239 | $1\,^4A_2$<br>$1\,^4A_2$ | 46.12<br>53.25 |
| $1\,^4A_2(D_{\infty h})$ | −164.998<br>−199.354 | 34.357 | $2\,^4B_1$<br>$2\,^4B_1$ | 46.12<br>53.25 |
| $1\,^4B_2(D_{\infty h})$ | −19.333<br>58.892 | 78.225 | $1\,^4B_1$<br>$1\,^4A_1$ | 36.74<br>38.87 |
| $2\,^4A_1(D_{\infty h})$ | −0.854<br>−0.132 | 0.722 | $2\,^4A_2$<br>$2\,^4A_2$ | 67.14<br>22.38 |

Table S.XV. Survey of spin-orbit coupling (SOC) effects (calculated at MRCI(ECP+CPP)/UET15 level of theory) for the previously shown extremal points (in the $C_{2v}$ subspace) of the **doublet** states of $Rb_3$ in **triangular configuration** (i.e. $D_{3h}$ or $C_{2v}$). SOC leads to an energy rising or lowering of the degenerate Kramers pair. Energies are given as the difference between SO results $E$ and the corresponding unperturbed energies $E_0$.

| State (geom.) | $E - E_0$ [cm$^{-1}$] | dominant couplings | strength [cm$^{-1}$] |
|---|---|---|---|
| $1\,^2B_1(C_{2v})$ | −0.4450 | $1\,^2B_2$ | 33.16 |
| $1\,^2A_1(C_{2v})$ | −0.588 | $1\,^2B_2$ | 36.01 |
| $1\,^2B_2(C_{2v})$ | 0.9964 | $1\,^2A_1$ | 49.07 |
| $2\,^2A_1(C_{2v})$ upper | 0.9760 | $2\,^2B_2$ | 41.21 |
| $3\,^2A_1(D_{3h})$ | −1.1198 | $1\,^2A_2$ | 38.59 |
| $1\,^2A_2(C_{2v})$ | 0.3728 | $2\,^2A_1$ | 41.66 |
| $2\,^2B_2(C_{2v})$ | 0.064 43 | $2\,^2A_1$ | 44.48 |
| $4\,^2A_1(C_{2v})$ lower | 0.2481 | $2\,^2B_1$ | 32.86 |
| $4\,^2A_1(C_{2v})$ upper | 0.6338 | $2\,^2B_1$ | 33.36 |

Table S.XVI. Survey of spin-orbit coupling (SOC) effects (calculated at MRCI(ECP+CPP)/UET15 level of theory) for the previously shown extremal points (in the $C_{2v}$ subspace) of the **doublet** states of $Rb_3$ in **linear configuration** (i.e. $D_{\infty h}$). SOC leads to an energy rising or lowering of the degenerate Kramers pair. Energies are given as the difference between SO results $E$ and the corresponding unperturbed energies $E_0$.

| State (geom.) | $E - E_0$ [cm$^{-1}$] | dominant couplings | strength [cm$^{-1}$] |
|---|---|---|---|
| $1\,^2B_1(D_{\infty h})$ | −0.1687 | $1\,^4B_2$ | 25.54 |
| $1\,^2A_1(D_{\infty h})$ | −0.2102 | $2\,^4A_2$ | 31.93 |
| $2\,^2A_1(D_{\infty h})$ | −3.1113 | $1\,^2A_2$ | 39.28 |
| $1\,^2B_2(D_{\infty h})$ | −73.9239 | $2\,^2A_1$ | 75.16 |
| $3\,^2A_1(D_{\infty h})$ | 67.8894 | $1\,^2B_2$ | 69.11 |
| $1\,^2A_2(D_{\infty h})$ | −34.2703 | $3\,^2A_1$ | 44.09 |
| $3\,^2B_1(D_{\infty h})$ | −0.6701 | $2\,^2B_2$ | 39.75 |
| $4\,^2B_1(D_{\infty h})$ | 7.3173 | $1\,^4B_2$ | 27.99 |
| $4\,^2A_1(D_{\infty h})$ | −0.038 12 | $3\,^4A_2$ | 23.64 |

## ROTATIONAL CONSTANTS FROM THE RIGID ROTOR APPROXIMATION

From the rigid rotor approximation we can define rotational term energies. They scale with their corresponding rotational constants, in general given as

$$A_x = \frac{\hbar}{4\pi c \Theta_x} \tag{S24a}$$

$$A_y = \frac{\hbar}{4\pi c \Theta_y} \tag{S24b}$$

$$A_z = \frac{\hbar}{4\pi c \Theta_z} \,, \tag{S24c}$$

with $\Theta_i \, , i \in \{x, y, z\}$ the principal moments of inertia, i.e. the eigenvalues of the inertia tensor

$$\Theta_{ij} = \sum_{k=1}^{N} m_k \left( \|\mathbf{r}\|^2 \delta_{ij} - x_i x_j \right) \,. \tag{S25}$$

This is a real symmetric rank-2 tensor which can be always diagonalized yielding the eigenvalues $\Theta_i$.

In principal it is only useful to calculate the inertia tensor with respect to the centre of mass. However our molecule fixed coordinate system $K'$ in Fig. 2 (of the main text) is not identical with the centre of mass system $K$. This means for obtaining the »correct« principal moments of inertia for calculating the rotational constants according to Eqs. (S24) we have to either account for the parallel axis theorem or transform to the center of mass system first. In the center of mass system the inertia tensor is diagonal with

$$\Theta_x = \frac{2}{3} m \left( R_{12}^2 - \frac{R_{23}^2}{4} \right) = \frac{2}{3} m \left( R_{13}^2 - \frac{R_{23}^2}{4} \right) \tag{S26a}$$

$$\Theta_y = \frac{1}{3} m \left( R_{12}^2 + R_{23}^2 \right) = \frac{1}{3} m \left( R_{13}^2 + R_{23}^2 \right) \tag{S26b}$$

$$\Theta_z = \frac{1}{2} m R_{23}^2 \,. \tag{S26c}$$

From this we can easily see the characteristic behaviour for equilateral triangular configurations and linear geometries. In this case we obtain symmetric rotators with $\Theta_x = \Theta_z$, respectively $\Theta_x = 0; \Theta_y = \Theta_z$. As $\Theta_x = 0$ for linear $D_{\infty h}$ configurations the corresponding rotational constant $A_x$ is undefined.

Table S.XVII. Synopsis of rotational constants for $^{87}$Rb for doublet and quartet states of $Rb_3$ in **triangular** configurations.

| State ($D_{3h}$) | $R_{12}, R_{23}, R_{13}$ [Å] | Geometry | $A_x$ [cm$^{-1}$] | $A_y$ [cm$^{-1}$] | $A_z$ [cm$^{-1}$] | Classification |
|---|---|---|---|---|---|---|
| $1\,^4B_1$ ($1\,^4A_2'$) | $5.311, 5.311, 5.311$ | $D_{3h}$ | 1.38 | 0.69 | 1.38 | symmetric rotor |
| $1\,^4A_2$ ($1\,^4E''$) | $4.368, 5.700, 4.368$ | $C_{2v}$ | 2.66 | 0.82 | 1.19 | asymmetric rotor |
| $2\,^4B_1$ ($1\,^4E'$) | $4.442, 8.179, 4.442$ | $C_{2v}$ | 9.68 | 0.55 | 0.58 | asymmetric rotor |
| $1\,^4A_1$ ($1\,^4E'$) | $4.993, 8.076, 4.993$ | $C_{2v}$ | 3.38 | 0.51 | 0.59 | asymmetric rotor |
| $2\,^4A_1$ ($1\,^4A_1'$) | $5.325, 5.325, 5.325$ | $D_{3h}$ | 1.37 | 0.68 | 1.37 | symmetric rotor |
| $3\,^4B_1$ ($2\,^4A_2'$) | $5.084, 5.084, 5.084$ | $D_{3h}$ | 1.50 | 0.75 | 1.50 | symmetric rotor |
| $2\,^4B_2$ ($2\,^4E''$) | $4.443, 6.217, 4.443$ | $C_{2v}$ | 2.89 | 0.74 | 1.00 | asymmetric rotor |
| $4\,^4B_1$ ($2\,^4E'$) | $5.283, 5.337, 5.283$ | $C_{2v}$ | 1.40 | 0.69 | 1.36 | asymmetric rotor |
| $3\,^4A_1$ (upper) ($2\,^4E'$) | $4.687, 7.226, 4.687$ | $C_{2v}$ | 3.27 | 0.61 | 0.74 | asymmetric rotor |
| $1\,^2B_1$ ($1\,^2E'$) | $4.379, 5.393, 4.379$ | $C_{2v}$ | 2.44 | 0.86 | 1.33 | asymmetric rotor |
| $1\,^2B_2$ ($1\,^2A_2''$) | $4.276, 4.285, 4.276$ | $C_{2v}$ | 2.12 | 1.06 | 2.11 | asymmetric rotor |
| $2\,^2A_1$ ($2\,^2E'$) | $4.398, 6.073, 4.398$ | $C_{2v}$ | 2.87 | 0.77 | 1.05 | asymmetric rotor |
| $3\,^2A_1$ ($1\,^2A_1'$) | $4.557, 4.557, 4.557$ | $D_{3h}$ | 1.87 | 0.93 | 1.87 | symmetric rotor |
| $1\,^2A_2$ ($1\,^2E''$) | $4.337, 5.132, 4.337$ | $C_{2v}$ | 2.38 | 0.91 | 1.47 | asymmetric rotor |
| $1\,^1A_1$ ($^1A_1'$) | $4.610, 4.610, 4.610$ | $D_{3h}$ | 1.82 | 0.91 | 1.82 | symmetric rotor |

Table S.XVIII. Synopsis of rotational constants for $^{87}$Rb for doublet and quartet states of $Rb_3$ in **linear** configurations.

| State ($D_{\infty h}$) | $R_{12}, R_{23}, R_{13}$ [Å] | $A_x$ [cm$^{-1}$] | $A_y$ [cm$^{-1}$] | $A_z$ [cm$^{-1}$] | Classification |
|---|---|---|---|---|---|
| $1\,^4A_2 + 2\,^4B_1 (1\,^4\Pi_g)$ | 4.435, 8.869, 4.435 | – | 0.493 | 0.493 | symmetric rotor |
| $2\,^4A_1 (1\,^4\Sigma_g^+)$ | 4.937, 9.874, 4.937 | – | 0.398 | 0.398 | symmetric rotor |
| $1\,^2A_1\ (1\,^2\Sigma_g^+)$ | 4.795, 9.590, 4.795 | – | 0.422 | 0.422 | symmetric rotor |
| $3\,^2A_1\ (2\,^2\Sigma_g^+)$ | 4.440, 8.880, 4.440 | – | 0.492 | 0.492 | symmetric rotor |
| $3\,^2B_1\ (2\,^2\Sigma_u^+)$ | 4.930, 9.860, 4.930 | – | 0.399 | 0.399 | symmetric rotor |
| $1\,^3B_1\ (^3\Sigma_u^+)$ | 4.875, 9.749, 4.875 | – | 0.408 | 0.408 | symmetric rotor |

*Note:* The data corresponding to the Figures shown here are also available in this supplementary material.


[S1] I. S. Lim, P. Schwerdtfeger, B. Metz, and H. Stoll, J. Chem. Phys. **122**, 104103 (2005).
[S2] A. W. Hauser, G. Auböck, C. Callegari, and W. E. Ernst, J. Chem. Phys. **132**, 164310 (2010).
[S3] P. Soldán, J. Chem. Phys. **132**, 234308 (2010).
[S4] S. Huzinaga and B. Miguel, Chem. Phys. Lett. **175**, 289 (1990).
[S5] S. Huzinaga and M. Klobukowski, Chem. Phys. Lett. **212**, 260 (1993).
[S6] D. P. Tew and W. Klopper, J. Chem. Phys. **125**, 094302 (2006).
[S7] I. Cherkes, S. Klaiman, and N. Moiseyev, Int. J. Quantum Chem. **109**, 2996 (2009).
[S8] H. Silberbach, P. Schwerdtfeger, H. Stoll, and H. Preuss, J. Phys. B: At. Mol. Phys. **19**, 501 (1986).
[S9] P. J. Linstrom and W. G. Mallard, "NIST Chemistry WebBook, NIST Standard Reference Database Number 69," (2019), data retrieved `https://doi.org/10.18434/T4D303`.
[S10] F. Cocchini, T. H. Upton, and W. Andreoni, J. Chem. Phys. **88**, 6068 (1988).
[S11] C. M. R. Rocha and A. J. C. Varandas, J. Chem. Phys. **144**, 064309 (2016).
[S12] I. B. Bersuker, Chem. Rev. **101**, 1067 (2001).
[S13] I. B. Bersuker, Chem. Rev. **113**, 1351 (2013).
[S14] A. W. Hauser, C. Callegari, P. Soldán, and W. E. Ernst, Chem. Phys. **375**, 73 (2010).
[S15] A. W. Hauser, C. Callegari, and W. E. Ernst, "Level-structure and magnetic properties from one-electron atoms to clusters with delocalized electronic orbitals: Shell models for alkali trimers," in *Advances in the Theory of Atomic and Molecular Systems: Dynamics, Spectroscopy, Clusters, and Nanostructures* (Springer Netherlands, Dordrecht, 2009) pp. 201–215.
[S16] A. W. Hauser, *The electronic structure of alkali trimers in their doublet and quartet manifolds: shell models and quantum chemistry calculations*, Ph.D. thesis, Technische Universität Graz (2009).
[S17] Y. Liu, I. B. Bersuker, W. Zou, and J. E. Boggs, Chem. Phys. **376**, 30 (2010).
[S18] D. Bishop, *Group Theory and Chemistry*, Dover books on physics and chemistry (Dover, 1993).
